# Supplementary material for: Accelerating Unified Multimodal Models with Core-Expansion Routing and Unified Computation Scheduling
Source: arXiv:2608.29291 source file (2026-12-01)
Supplement: Supplementary file 1 [file appendix.tex]

\section{Hello World}
%\subsection{Hello World}
